# Supplementary material for: Diverse Teacher-Students for Deep Safe Semi-Supervised Learning under Class Mismatch
Source: arXiv:2405.16093 source file (2024-05-25)
Supplement: Supplementary file 1 [file X_suppl.tex]

\section{Supplementary Material}
